# Supplementary material for: Diversity Policy Gradient for Sample Efficient Quality-Diversity Optimization
Source: arXiv:2006.08505 source file (2022-05-31)
Supplement: Supplementary file 1 [file sm_pseudocode.tex]

\makeatletter
\makeatother

\SetKwComment{Comment}{/* }{ */}

\begin{algorithm}
    \small
    \SetAlgoLined
    \DontPrintSemicolon
    \SetKwInput{KwInput}{Given}
    \KwInput{N, max\_steps, gradient\_steps G, BD and state descriptor extraction functions extraction functions $\xi$, $\psi$}
    \SetKwInput{KwInput}{Initialize}
    \KwInput{MAP-Elites grid $\mathbb{M}$, Replay Buffer $\mathbb{B}$, $N$ actors $\{\pi_{\theta_{i}}\}_{i=\{1,\dots,N\}}$, 2 critics $Q^D_w$, $Q^Q_w$, state descriptors archive $\mathbb{A}$}\;
    $\textrm{total\_steps}, \textrm{actor\_steps} = 0, 0 $ \tcp*{Step counters}\;
    $\textrm{initialisation} = True$ \tcp*{Step counters}\;

    \While(\tcp*{Main loop}){$total\_steps<max\_steps$}{
        
        \If{$\textrm{not}~ \textrm{initialisation}$}{
            Select generation $\{\pi_{\theta_i}\}_{i = 1, \dots, N}$ from grid $\mathbb{M}$
            
            \For(\tcp*[f]{Population update}){$i \leftarrow 1$ \KwTo $G$}{
                \tcp{Update actors and critic for diversity}
                Compute novelty rewards as $r^D_t$ from $\psi(s_t)$ and $\mathbb{A}$\;
                Update novelty critic $Q^D_{w}$\;
                Update $\{\pi_{\theta_i}\}_{i \leq N//2}$ for diversity using $Q^D_{w}$\;

                $\{\pi_{\theta_i}\}_{i \leq N//2}, Q^D_{w} \leftarrow \textrm{update}(\{\pi_{\theta_i}\}_{i \leq N//2}, Q^D_{w}, \mathbb{B}, \mathbb{A})$
                
                \tcp{Update actors and critic for quality}
                $\{\pi_{\theta_i}\}_{i > N//2}, Q^Q_{v} \leftarrow \textrm{update}(\{\pi_{\theta_i}\}_{i > N//2}, Q^Q_{v}, \mathbb{B})$
            }
        }

        \For(\tcp*{Population evaluation}){$j \leftarrow 1$ \KwTo N}{
        
            Play one episode with actor $\pi_{\theta_{j}}$\ and store all transitions in $\mathbb{B}$\;
            Get episode length $T$, discounted return $R$ and state descriptors $\{\psi(s_1), \dots, \psi(s_T)\}$\;
            Store state descriptors $\{\psi(s_1), \dots, \psi(s_T)\}$ in $\mathbb{A}$\;
            Compute $\xi(\theta_j)$ and add the tuple ($R$, $\xi(\theta_j)$, $\theta_j$) in the MAP-Elites grid $\mathbb{M}$\;
            $actor\_steps \leftarrow actor\_steps + T$\;
        
            $\{(s_t, a_t, r_t, s_{t+1}, \psi(s_t))\}_{t = 1, \dots, T} \leftarrow \textrm{evaluate}(\pi_{\theta_{j}})$
            $f(\theta_{j}), \xi(\theta_{j}) \leftarrow \textrm{compute}(\{(s_t, a_t, r_t, s_{t+1}, \psi(s_t))\}_{t})$
            $\mathbb{M} \leftarrow \textrm{add}(\mathbb{M}, f(\theta_{j}), \xi(\theta_{j}), \xi(\theta_{j}))$
            $\mathbb{B} \leftarrow \textrm{store}(\mathbb{B}, \{(s_t, a_t, r_t, s_{t+1}, \psi(s_t))\}_{t})$
            $\mathbb{A} \leftarrow \textrm{store}(\mathbb{A}, \{\psi(s_t)\}_{t = 1, \dots, T})$
        
            $actor\_steps \leftarrow actor\_steps + T$\;
        }

        $total\_steps \leftarrow total\_steps + actor\_steps$ \tcp{Update total time steps}\;
    }

    \caption{QD-PG}
    \label{alg:compact_pseudocode}
\end{algorithm}
